# Supplementary material for: Ins-HOI: Instance Aware Human-Object Interactions Recovery
Source: arXiv:2312.09641 source file (2024-03-21)
Supplement: Supplementary file 1 [file 7_Appendix.tex]

\section{More Implementation Details}

\paragraph{Attention Module.}
We follow Mesh Graphormer~\cite{lin2021mesh} to implement the attention module for the grid and mesh-aligned feature fusion.
We simply use a single attention block for each iteration because we found that a single block brought enough performance grains while using more attention blocks merely increased memory consumption.

\paragraph{Mesh Sampling.}
For body and hand meshes, we simply use the down-sampling matrix provided in GraphCMR~\cite{kolotouros2019convolutional} and Mesh Graphormer~\cite{lin2021mesh} to reduce the vertex number for mesh-aligned feature extraction.
For face meshes, we manually select the vertices in the front face region considering that the expression information concentrates on the front face.
For body-only PyMAF, the dimension of the mesh-aligned features is reduced to match the feature dimension in HMR~\cite{kanazawa2018end} for more fair comparisons.
For hand- and face-only PyMAF, we do not strictly abide by this rule but simply replace SMPL with MANO/FLAME during the implementation.
Fig.~\ref{fig:sampling_mesh} visualizes the selected vertices on the body, hand, and face meshes.

\begin{figure}[t]
	\centering
	\includegraphics[width=0.5\textwidth]{fig/vis/sampling_mesh.pdf}
    \vspace{-5mm}
	\caption{Visualization of the selected vertices on the body, hand, and face models for mesh-aligned feature extraction.}
	\label{fig:sampling_mesh}
\end{figure}

\begin{figure}[t]
	\centering
	\includegraphics[width=0.5\textwidth]{fig/vis/vis_dense_map.pdf}
    \vspace{-5mm}
	\caption{Visualization of the rendered dense correspondences in resolutions of $56 \times 56$ for the body, hand, and face meshes. From left to right: the IUV~\cite{guler2018densepose} map for a body model, the PNCC~\cite{zhu2017face} maps for hand and face models.}
    \vspace{-5mm}
	\label{fig:vis_dense_map}
\end{figure}

\paragraph{Auxiliary Dense Supervision.}
In the auxiliary dense prediction task, the dense correspondence and part segmentation (for ablation experiments) used for supervision are rendered based on the pseudo ground truth meshes.
Examples of the rendered dense correspondence are visualized in Fig.~\ref{fig:vis_dense_map}.
We choose to use the rendered dense correspondence mainly based on the following reasons:

i) The dense correspondence can be regarded as a more fine-grained part segmentation. In our method, we use the IUV representation as dense correspondence for the body expert, while using the Projected Normalized Coordinate Code (PNCC)~\cite{zhu2017face} for hand and face experts.
% Note that the dense correspondence is not limited to the IUV representation. The Projected Normalized Coordinate Code (PNCC)~\cite{zhu2017face} can be also used as dense correspondence. 
% From this perspective, 
Dense correspondences are more general since PNCC does not need to split the mesh into manually defined parts.

ii) The body part definition may vary from different datasets while the rendered one is consistent. Moreover, the rendering process can be done efficiently in batch using the tools like PyTorch3D~\cite{ravi2020accelerating}. The costs of rendering part segmentation and dense correspondences are almost the same for the PyTorch3D renderer.

iii) There is only a limited number of datasets providing the annotated part segmentation and dense correspondence, while the pseudo ground truth meshes are typically available for common datasets thanks to previous work such as SPIN~\cite{kolotouros2019learning} and EFT~\cite{joo2021exemplar}.

\paragraph{Hand Visibility.}
We simply use three FC layers to predict hand visibility based on the hand-only mesh-aligned features. The pseudo visibility confidence used for supervision is calculated based on the proportion of the visible hand keypoints annotated in the whole-body COCO~\cite{jin2020whole} dataset.
For example, assume that there are 15 visible keypoints and the total number of hand keypoints is 21, then the pseudo visibility confidence of this hand is about 0.714 (15/21).

\section{About Metrics}
Though the PA-PVE and PA-MPJPE are widely adopted in the 3D pose estimation task, these two metrics can not fully reveal the mesh-image alignment performance since they are calculated after rigid alignment.
As depicted in Fig.~\ref{fig:metrics}, a reconstruction result with a lower PA-MPJPE value can have a higher MPJPE value and worse alignment between the reprojected mesh and image.

\begin{figure}[t]
	\centering
	\begin{subfigure}[b]{0.23\textwidth}
		\includegraphics[width=1\textwidth]{fig/vis/metric/bad.png}
		\caption{\scriptsize PA-MPJPE: 26.9, MPJPE: 74.3}
		\label{fig:bad}
    \end{subfigure}
	\begin{subfigure}[b]{0.23\textwidth}
		\includegraphics[width=1\textwidth]{fig/vis/metric/good.png}
		\caption{\scriptsize PA-MPJPE: 27.7, MPJPE: 43.4}
		\label{fig:good}
    \end{subfigure}
    \vspace{-2mm}
	\caption{Examples of two reconstruction results. (a) A reconstruction result with a lower PA-MPJPE value but worse mesh-image alignment. (b) A reconstruction result with a higher PA-MPJPE value but better mesh-image alignment.}
	\label{fig:metrics}
\end{figure}

\section{About Datasets}
\label{sec:datasets}
Following the practices of previous work~\cite{kanazawa2018end,kolotouros2019learning,kocabas2021pare}, we train our body model regression network on several datasets with 3D or 2D annotations, including Human3.6M~\cite{ionescu2014human3}, MPI-INF-3DHP~\cite{mehta2017monocular}, LSP~\cite{johnson2010clustered}, MPII~\cite{andriluka20142d}, COCO~\cite{lin2014microsoft}.
For hand-only and full-body model regression, FreiHAND~\cite{zimmermann2019freihand}, InterHand2.6M~\cite{moon2020interhand2}, FFHQ~\cite{karras2019style}, and COCO-WholeBody~\cite{jin2020whole} are also used for training.
Here, we provide more descriptions of the datasets to supplement the main manuscript.

\textbf{Human3.6M}~\cite{ionescu2014human3} is commonly used as the benchmark dataset for 3D human pose estimation, consisting of 3.6 million video frames captured in the controlled environment.
The ground truth SMPL parameters in Human3.6M are generated by applying MoSH~\cite{loper2014mosh} to the sparse 3D MoCap marker data, as done in Kanazawa \etal~\cite{kanazawa2018end}.
The original videos are down-sampled from 50fps to 10fps, resulting in 312,188 frames for training.
Following the common protocols~\cite{pavlakos2017coarse,pavlakos2018learning,kanazawa2018end}, our experiments use five subjects (S1, S5, S6, S7, S8) for training and two subjects (S9, S11) for evaluation.
The original videos are also down-sampled from 50 fps to 10 fps to remove redundant frames, resulting in 312,188 frames for training and 26,859 frames for evaluation.

\textbf{3DPW}~\cite{von2018recovering} is captured in challenging outdoor scenes with IMU-equipped actors under various activities.
This dataset provides accurate shape and pose ground truth annotations.
Following the protocol of previous work~\cite{kanazawa2019learning,kolotouros2019learning}, we do not use its data for training by default unless specified in the table.

\textbf{MPI-INF-3DHP}~\cite{mehta2017monocular} is a 3D human pose dataset covering more actor subjects and poses than Human3.6M.
The images of this dataset were collected under both indoor and outdoor scenes, and the 3D annotations were captured by a multi-camera marker-less MoCap system.
Hence, there is some noise in the 3D ground truth annotations.
The training set includes 8 subjects and there are 96,507 frames down-sampled from videos used for training.
% The test set consists of 2,875 valid frames covering 7 activities performed by 6 subjects.

\textbf{LSP}~\cite{johnson2010clustered} and \textbf{LSP-Extended}~\cite{johnson2011learning} are 2D human pose benchmark datasets, containing person images with challenging poses. There are 14 visible 2D keypoint locations annotated for each image and 10,428 samples used for training.

\textbf{MPII}~\cite{andriluka20142d} is a standard benchmark for 2D human pose estimation.
There are 25,000 images collected from YouTube videos covering a wide range of activities.
We discard those images without complete keypoint annotations, producing 14,667 samples for training.

\textbf{COCO}~\cite{lin2014microsoft} and \textbf{COCO-WholeBody}~\cite{jin2020whole} contain a large scale of person images labeled with 17 body keypoints, 42 hand keypoints, and 68 face keypoints.
We use COCO to train body-only PyMAF and leverage the hand keypoints in COCO-WholeBody during the training of hand- and face-only PyMAF and PyMAF-X.
Since this dataset does not contain ground-truth meshes, we conduct a quantitative evaluation on the 2D keypoint localization task using its validation set, which consists of 50,197 samples.

\textbf{EHF}~\cite{pavlakos2019expressive} contains 100 testing images of one subject captured in lab environments.
For each image, the corresponding 3D scans and ground-truth SMPL-X~\cite{pavlakos2019expressive} meshes are provided.
EHF is used for testing only and is commonly adopted as a full-body evaluation benchmark dataset in literature~\cite{choutas2020monocular,feng2021collaborative,moon2022Hand4Whole}.

\textbf{AGORA}~\cite{patel2021agora} is a synthetic dataset with accurate SMPL-X models fitted to 3D scans.
Since the ground-truth labels of its test set are not publicly available, the evaluation is performed on the official platform\footnote{\url{https://agora-evaluation.is.tuebingen.mpg.de}}.
For evaluation on AGORA, we use the training set of AGORA to finetune our model.

\textbf{FreiHAND}~\cite{zimmermann2019freihand} contains 130,240 samples for training and 3960 samples images for evaluation. For each sample in the training set, the MANO~\cite{romero2017embodied} parameters recovered from multi-view images are provided. We use this dataset for the training and evaluation of the hand expert.

\textbf{InterHand2.6M}~\cite{moon2020interhand2} is a large-scale real-captured hand dataset, providing accurate MANO parameters of interacting hands. We crop single-hand images from this dataset for the training of the hand expert.

% \textbf{FFHQ}~\cite{karras2019style} consists of 70,000 high-quality images of human faces.
% The facial landmarks are obtained via the method of Bulat \etal~\cite{bulat2017far} and used for the training of the face expert.

{

\textbf{VGGFace2}~\cite{Cao2018_VGGFace2} is a large-scale face dataset. The images of this dataset are downloaded from Google and have large variations in pose, age, and ethnicity. It contains about 3 million images from training.
We run the method of FAN~\cite{bulat2017far} and DECA~\cite{DECA_2020} on its training set to generate the pseudo ground truth facial landmarks and FLAME~\cite{li2017learning} models for the training of the face expert.

\textbf{Stirling3D}~\cite{Feng2018evaluation} provides facial images with the ground-truth 3D scans. The test set contains 2,000 facial images in neutral expressions, including 1,344 low-quality (LQ) images and 656 high-quality (HQ) images. We follow previous work~\cite{choutas2020monocular,DECA_2020} to use it for evaluation only.

\textbf{NoW}~\cite{Sanyal2019_ringnet} contains the facial images captured with an iPhone X, and a separate 3D scan for each subject.
Its test set contains 1,702 images for evaluation.
Since the ground-truth scans of the test set are not publicly available, the evaluation is performed by following the instructions on the official website\footnote{\url{https://now.is.tue.mpg.de/index.html}}.
We follow previous work~\cite{choutas2020monocular,DECA_2020} to use this dataset for evaluation only.
}

\section{More Qualitative Results}
\label{sec:further_qualitative}

We provide more qualitative results of our method in this section.
In Fig~\ref{fig:loop}, we visualize the estimated meshes after each iteration, where it can be seen that PyMAF can correct the drift of body parts progressively and result in better-aligned human models.
In Fig.~\ref{fig:smpl_cocoDemo}, the body mesh recovery results of different methods on COCO are depicted for qualitative comparisons, where PyMAF convincingly performs better than competitors and our baseline by producing better-aligned and natural results.
In Fig.~\ref{fig:well-aligned}, we provide more full-body model reconstruction results on the COCO validation set, where PyMAF-X can produce well-aligned full-body model under challenging cases.
In Fig.\ref{fig:smplx_novel_view}, we further visualize the reconstructed full-body models from different viewpoints.

\textbf{Cases under Occlusions.} As pointed out in the main paper, the adaptive integration is not applicable when the hand part is invisible. To handle this, the visibility status of hands is also predicted by the hand expert in PyMAF-X.
In cases of invisible hands, the full-body model adopts the default hand poses and the wrist poses estimated by the body expert.
Fig.~\ref{fig:occlusion} shows the example results of PyMAF-X when the body or hands are occluded.
We can see that PyMAF-X produces reasonable full-body meshes under these cases.

\textbf{Failure Cases.}
Due to the rotational pose representation of the kinematic model, the full-body alignment of PyMAF-X heavily relies on the accuracy of body pose estimation. Moreover, the misalignment may also occur when the body shape is inaccurate since it affects the body bone length.
Besides, it is still challenging for PyMAF-X to handle challenging hand poses or interacting hands.
Fig.~\ref{fig:failed_cases} visualizes some erroneous results of our approach, where PyMAF-X produces misaligned results due to the issues mentioned above.

\begin{figure}[t]
	\centering
% 	\hspace{1mm}
% 	\hspace{0.5mm}
	\foreach \idx in {2,3,4,5} {
		\begin{subfigure}[h]{0.45\textwidth}
% 			\centering
    		\includegraphics[width=1\textwidth]{fig/vis/loop/vis_loop_\idx.pdf}
		\end{subfigure}
	}
	\\
	\begin{tikzpicture}[remember picture,overlay]
	\node[font=\fontsize{8pt}{8pt}\selectfont] at (-3,-0.2) {Image};
	\node[font=\fontsize{8pt}{8pt}\selectfont] at (-1.5,-0.2) {$M_0$};
 	\node[font=\fontsize{8pt}{8pt}\selectfont] at (-0,-0.2) {$M_1$};
	\node[font=\fontsize{8pt}{8pt}\selectfont] at (1.7,-0.2) {$M_2$};
	\node[font=\fontsize{8pt}{8pt}\selectfont] at (3.2,-0.2) {$M_3$};
	\end{tikzpicture}
	\vspace{1mm}
	\caption{Visualization of reconstruction results across different iterations in the feedback loop.}
	% \vspace{-5mm}
	\label{fig:loop}
\end{figure}

\begin{figure}[t]
	\centering
% 	\hspace{1mm}
	\begin{tikzpicture}[remember picture,overlay]
	\node[font=\fontsize{8pt}{8pt}\selectfont, rotate=90] at (0,3.5) {Image};
 	\node[font=\fontsize{8pt}{8pt}\selectfont, rotate=90] at (0,1.9) {SPIN~\cite{kolotouros2019learning}};
 	\node[font=\fontsize{8pt}{8pt}\selectfont, rotate=90] at (0,0.3) {PARE~\cite{kocabas2021pare}};
	\node[font=\fontsize{8pt}{8pt}\selectfont, rotate=90] at (0,-1.4) {Baseline};
	\node[font=\fontsize{8pt}{8pt}\selectfont, rotate=90] at (0,-3.0) {PyMAF};
	\end{tikzpicture}
% 	\hspace{0.5mm}
	\foreach \idx in {1,2,3,4,5} {
		\begin{subfigure}[h]{0.082\textwidth}
			\centering
			\foreach \sub in {0,1,2,3,4} {
    			\pgfmathsetmacro\imidx{int(\sub * 5 + \idx)}
    			\includegraphics[width=1.1\textwidth]{fig/vis/coco/coco_\imidx.pdf}
    % 			\vspace{1mm}
    		}
		\end{subfigure}
	}
	\vspace{-6mm}
	\caption{Qualitative comparison of reconstruction results on the COCO validation set.}
	\vspace{-2mm}
	\label{fig:smpl_cocoDemo}
\end{figure}

\begin{figure*}[t]
	\centering
% 	\hspace{1mm}
% 	\hspace{0.5mm}
	\foreach \idx in {1, 2, 3, 4, 5, 6, 7, 8, 9, 10, 11, 12, 13, 14, 15, 16, 17, 18, 19, 20, 21, 22, 23, 24, 25, 26, 27, 28, 29, 30, 31, 32, 33, 34, 35, 36} {
		\begin{subfigure}[h]{0.32\textwidth}
% 			\centering
    		\includegraphics[width=1\textwidth]{fig/vis/smplx/demo/well-aligned_\idx.pdf}
		\end{subfigure}
	}
	\\
	\vspace{1mm}
	\caption{More examples of the full-body mesh recovery results of PyMAF-X on the COCO validation set. Best viewed zoomed-in on a color screen.}
	\vspace{-5mm}
	\label{fig:well-aligned}
\end{figure*}

\begin{figure*}[t]
	\centering
% 	\hspace{1mm}
% 	\hspace{0.5mm}
	\foreach \idx in {1, 2, 3, 4, 5, 6, 7, 8, 9, 10, 11, 12, 13, 14, 15, 16} {
		\begin{subfigure}[h]{0.49\textwidth}
% 			\centering
    		\includegraphics[width=1\textwidth]{fig/vis/smplx/novel_view/novel_view_\idx.pdf}
      ~
		\end{subfigure}
	}
    \\
	% \vspace{-6mm}
	\caption{PyMAF-X results visualized from different viewpoints. For each example, from left to right: the input image, the overlay result, and the results with rotations around the vertical axis. Best viewed zoomed-in on a color screen.}
	\vspace{-2mm}
	\label{fig:smplx_novel_view}
\end{figure*}

\begin{figure*}[t]
	\centering
% 	\hspace{1mm}
% 	\hspace{0.5mm}
	\foreach \idx in {1, 2, 3, 4, 5, 6, 7, 8, 9} {
		\begin{subfigure}[h]{0.32\textwidth}
% 			\centering
    		\includegraphics[width=1\textwidth]{fig/vis/smplx/occlusion/occlusion_\idx.pdf}
		\end{subfigure}
	}
	\\
	\vspace{1mm}
	\caption{Example results of PyMAF-X when the body or hands are occluded. Samples come from the COCO validation set. Best viewed zoomed-in on a color screen.}
	\vspace{-5mm}
	\label{fig:occlusion}
\end{figure*}

\begin{figure*}[t]
	\centering
    \begin{subfigure}[b]{0.49\textwidth}
		\includegraphics[width=1\textwidth]{fig/vis/smplx/fail/fail_2.pdf}
		\caption{Inaccurate bone length (body shape)}
    \end{subfigure}
    \begin{subfigure}[b]{0.49\textwidth}
		\includegraphics[width=1\textwidth]{fig/vis/smplx/fail/fail_4.pdf}
		\caption{Inaccurate body pose}
    \end{subfigure}
    \\
    \vspace{2mm}
    \begin{subfigure}[b]{0.49\textwidth}
		\includegraphics[width=1\textwidth]{fig/vis/smplx/fail/fail_3.pdf}
		\caption{Challenging hand pose}
    \end{subfigure}
    \begin{subfigure}[b]{0.49\textwidth}
		\includegraphics[width=1\textwidth]{fig/vis/smplx/fail/fail_1.pdf}
		\caption{Interacting hands}
    \end{subfigure}
	\caption{Misaligned reconstructions of our approach. Misalignment comes from (a) inaccurate bone length (body shape), (b) inaccurate body pose, (c)(d) inaccurate hand poses under challenging hand poses, occlusions, and interactions. Samples come from the COCO validation set.
	}
	\vspace{-5mm}
	\label{fig:failed_cases}
\end{figure*}
